# Supplementary material for: The Devil is in the Prompts: De-Identification Traces Enhance Memorization Risks in Synthetic Chest X-Ray Generation
Source: arXiv:2502.07516 source file (2025-02-14)
Supplement: Supplementary file 1 [file appendix.tex]

\section{Appendix}

\subsection{Algorithm for Detecting Memorized Prompts in MIMIC-CXR}

Here, we present the algorithm for detecting memorized prompts in the MIMIC-CXR dataset. First, we extract the set of all unique prompts ($\mathcal{P}$) in the dataset. Next, using a stable diffusion pipeline ($\mathcal{M}$) derived from \textit{RadEdit} \cite{perez2024radedit}, we compute the text-conditional noise for all the prompts ($p \in \mathcal{P}$) with 50 inference steps and four generations per prompt. Finally, we quantify a memorization score ($d_{mem}$) for each prompt by averaging the text-conditional noise across all timesteps and generations. The procedure is outlined in algorithm \ref{alg:memorization_detection}.

\begin{algorithm}
\caption{Detecting Memorized Prompts in MIMIC-CXR}
\label{alg:memorization_detection}
\begin{algorithmic}[1]
\Require Text-to-image model $\mathcal{M}$ with text-encoder $T_E$, dataset $\mathcal{D}$, number of timesteps $T$
\Ensure Memorization score $d_{mem}$ for each prompt $p \in \mathcal{D}$
\State Extract unique prompts: $\mathcal{P} \leftarrow \text{Unique}(\mathcal{D})$

\For{each prompt $p$ in $\mathcal{P}$}
    % \State Generate initial noise $\eta_0 \sim \mathcal{N}(0, I)$
    \State Encode text prompt: $e_p \leftarrow T_E(p)$
    \State Encode null prompt: $e_{\emptyset} \leftarrow T_E(\emptyset)$
    % \State Initialize latent representation: $z_T \leftarrow V_E(\eta_0)$
    
    \For{$t = T$ to $1$}
        \State Predict noise (text prompt): $\hat{\eta_t} \leftarrow \epsilon_{\theta}(x_t, e_p)$
        \State Predict noise (null prompt): $\hat{\phi_t} \leftarrow \epsilon_{\theta}(x_t, e_{\emptyset})$
        % \State Update latent variable: $z_{t-1} \leftarrow z_t - \hat{\eta_t}$
        % \State Compute text-conditional noise metric: $d_{mem}(p) \leftarrow \sum_{t=1}^{T} ||\hat{\eta_t} - \eta_t||$
        \State Compute $d_{mem}(p, t) \leftarrow ||\hat{\eta_t} - \hat{\phi_t}||_2$
    \EndFor

    \State $d_{mem}(p) \leftarrow \frac{1}{T} \sum_{t=1}^T d_{mem}(p,t)$
\EndFor
\State \Return Memorization scores $\{d_{mem}(p)\}_{p \in \mathcal{D}}$

\end{algorithmic}
\end{algorithm}

\subsection{De-Identification Markers are Amongst the Most Memorized}

We compute the token-wise importance scores for all tokens in \textit{memorized prompts}. For each prompt, we show which tokens in the prompt contribute the most towards memorization. In each case, shown in Fig. \ref{fig:three_plots}, we find that the de-identification marker (\textunderscore\textunderscore\textunderscore) poses the highest memorization threat. We provide the following justifications for this:

\begin{enumerate}
    \item The de-identification marker is a distinct and unique token differing from all other tokens in the MIMIC-CXR dataset.
    \item Due to the de-identification process, its frequency is sufficient enough to create spurious correlations with certain samples and make associated text prompts highly specific.
    \item Highly specific text tokens and prompts can act as keys into the diffusion model's memory and enable retrieving certain data points during inference, indicating memorization.
\end{enumerate}

\begin{figure}[htbp]
    \centering
    
    \subfloat[\textbf{Prompt:} \textit{AP chest compared to \textcolor{red}{\textunderscore\textunderscore\textunderscore}: Previous mild pulmonary edema has resolved.  There is no pneumonia. Several small lung nodules and the large right paratracheal mediastinal mass are manifestations of lung cancer. Heart size normal.  No appreciable pleural effusion.}
    ]{
        \includegraphics[width=0.9\textwidth]{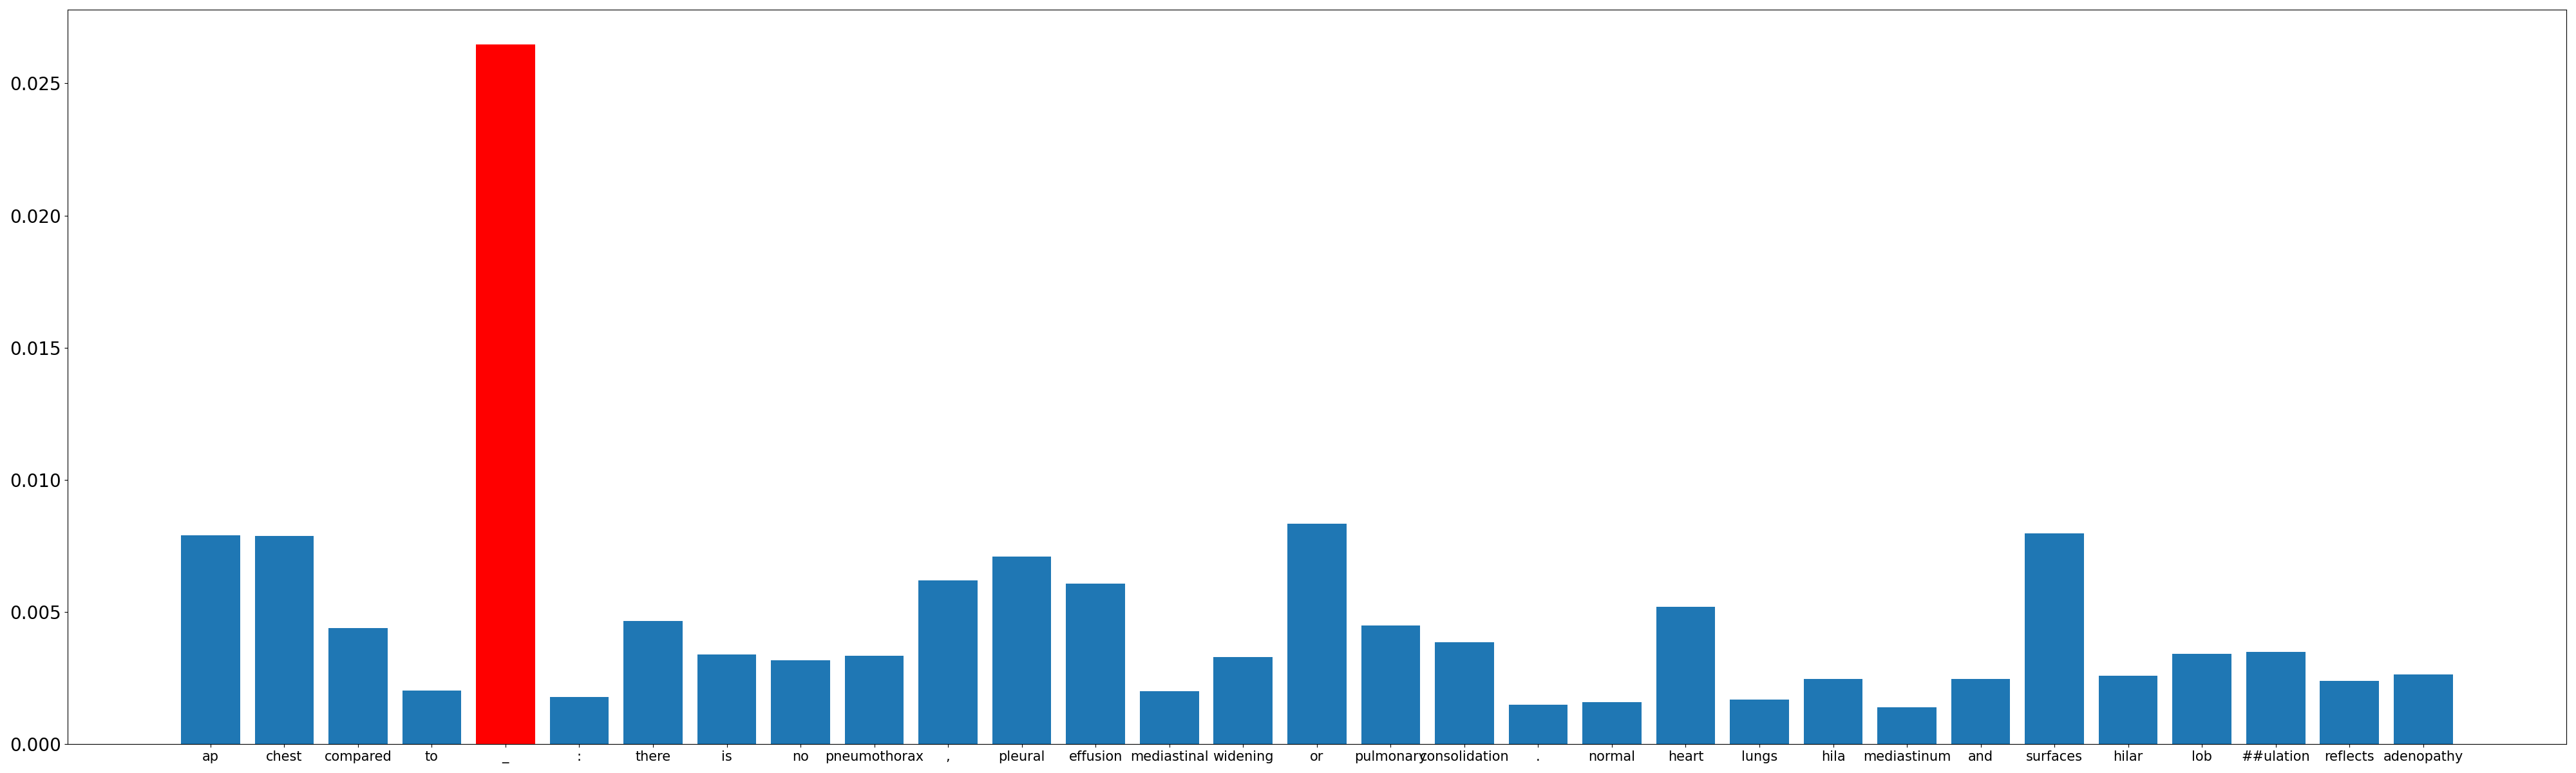}
    }
    
    \subfloat[\textbf{Prompt:} \textit{Comparison to \textcolor{red}{\textunderscore\textunderscore\textunderscore}: The 2 right-sided chest tubes are in stable position. Extensive soft tissue air collections bilaterally. The chest radiograph does not clearly show the presence of a pneumothorax. Stability in extent and severity of the bilateral parenchymal opacities at the lung bases. No pleural effusions.}
    ]{
        \includegraphics[width=0.9\textwidth]{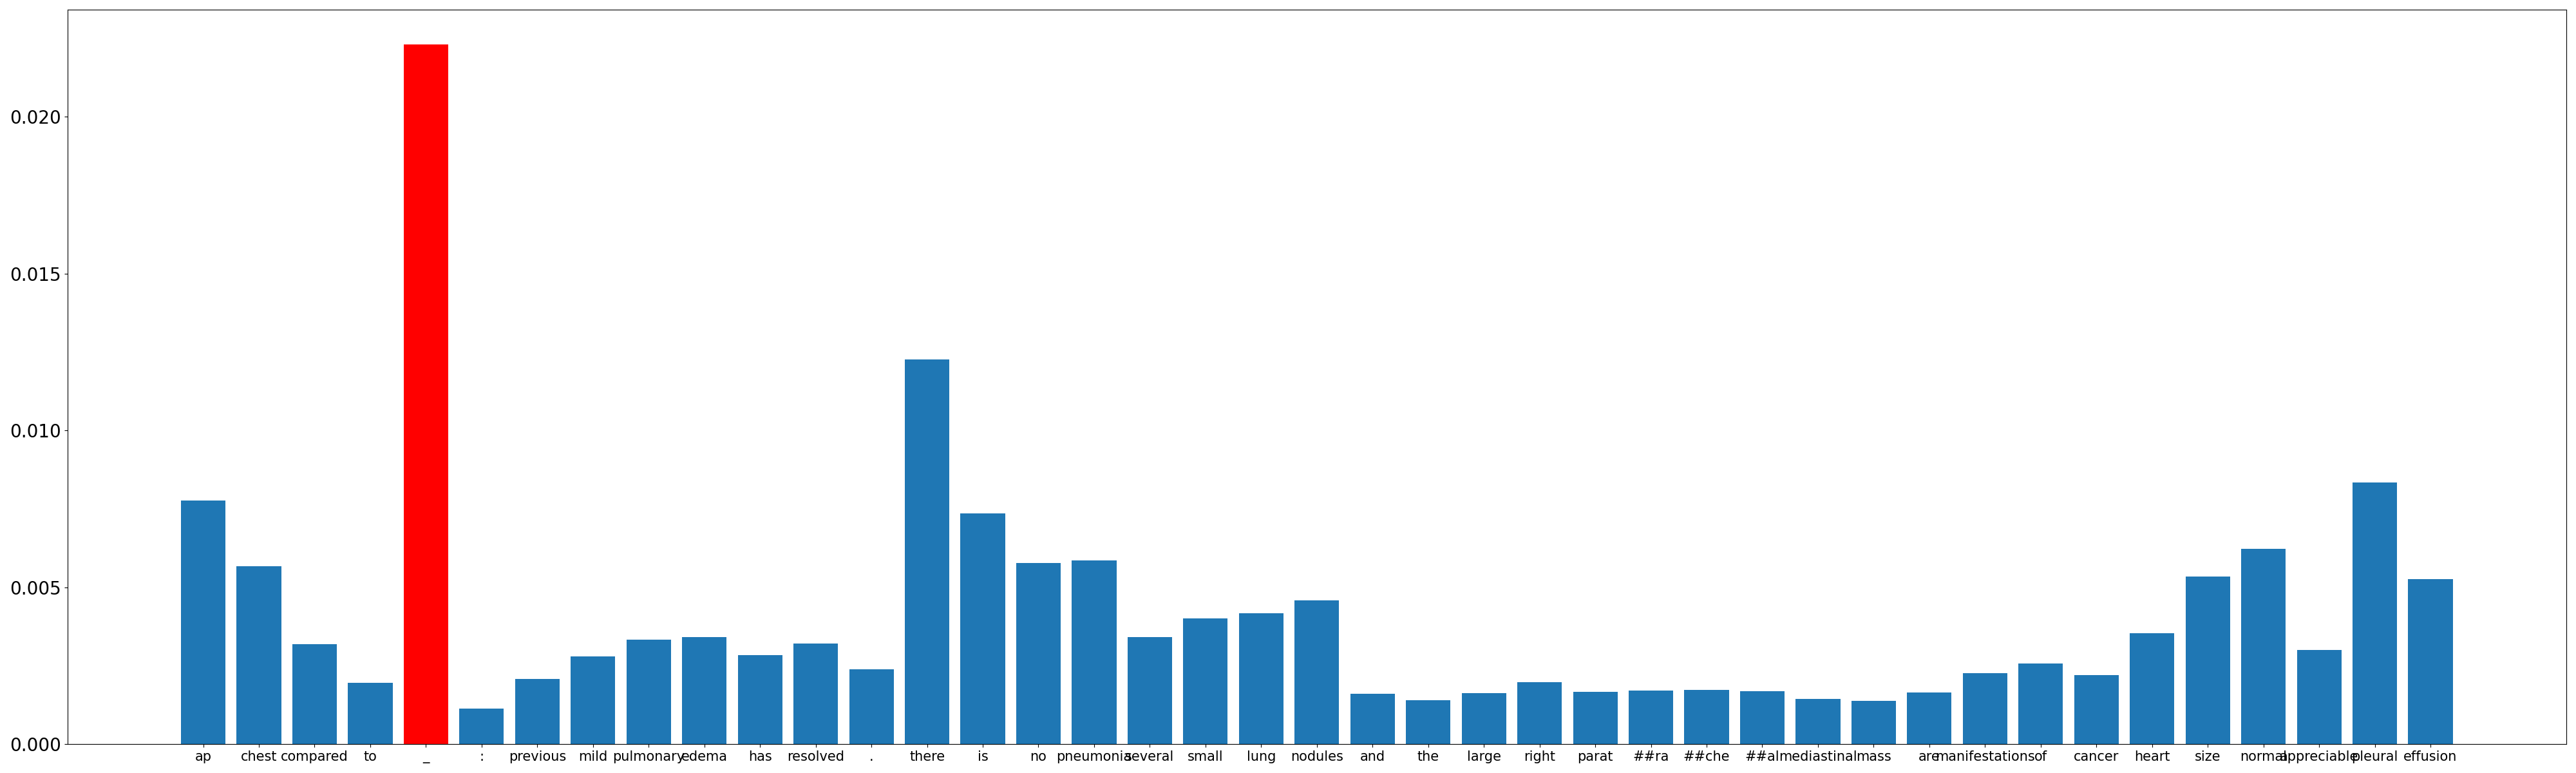}
    }
    
    \subfloat[\textbf{Prompt:} \textit{AP chest compared to \textcolor{red}{\textunderscore\textunderscore\textunderscore}: There is no pneumothorax, pleural effusion, mediastinal widening or pulmonary consolidation.  Normal heart, lungs, hila, mediastinum and pleural surfaces. Hilar lobulation reflects adenopathy.}
    ]{
        \includegraphics[width=0.9\textwidth]{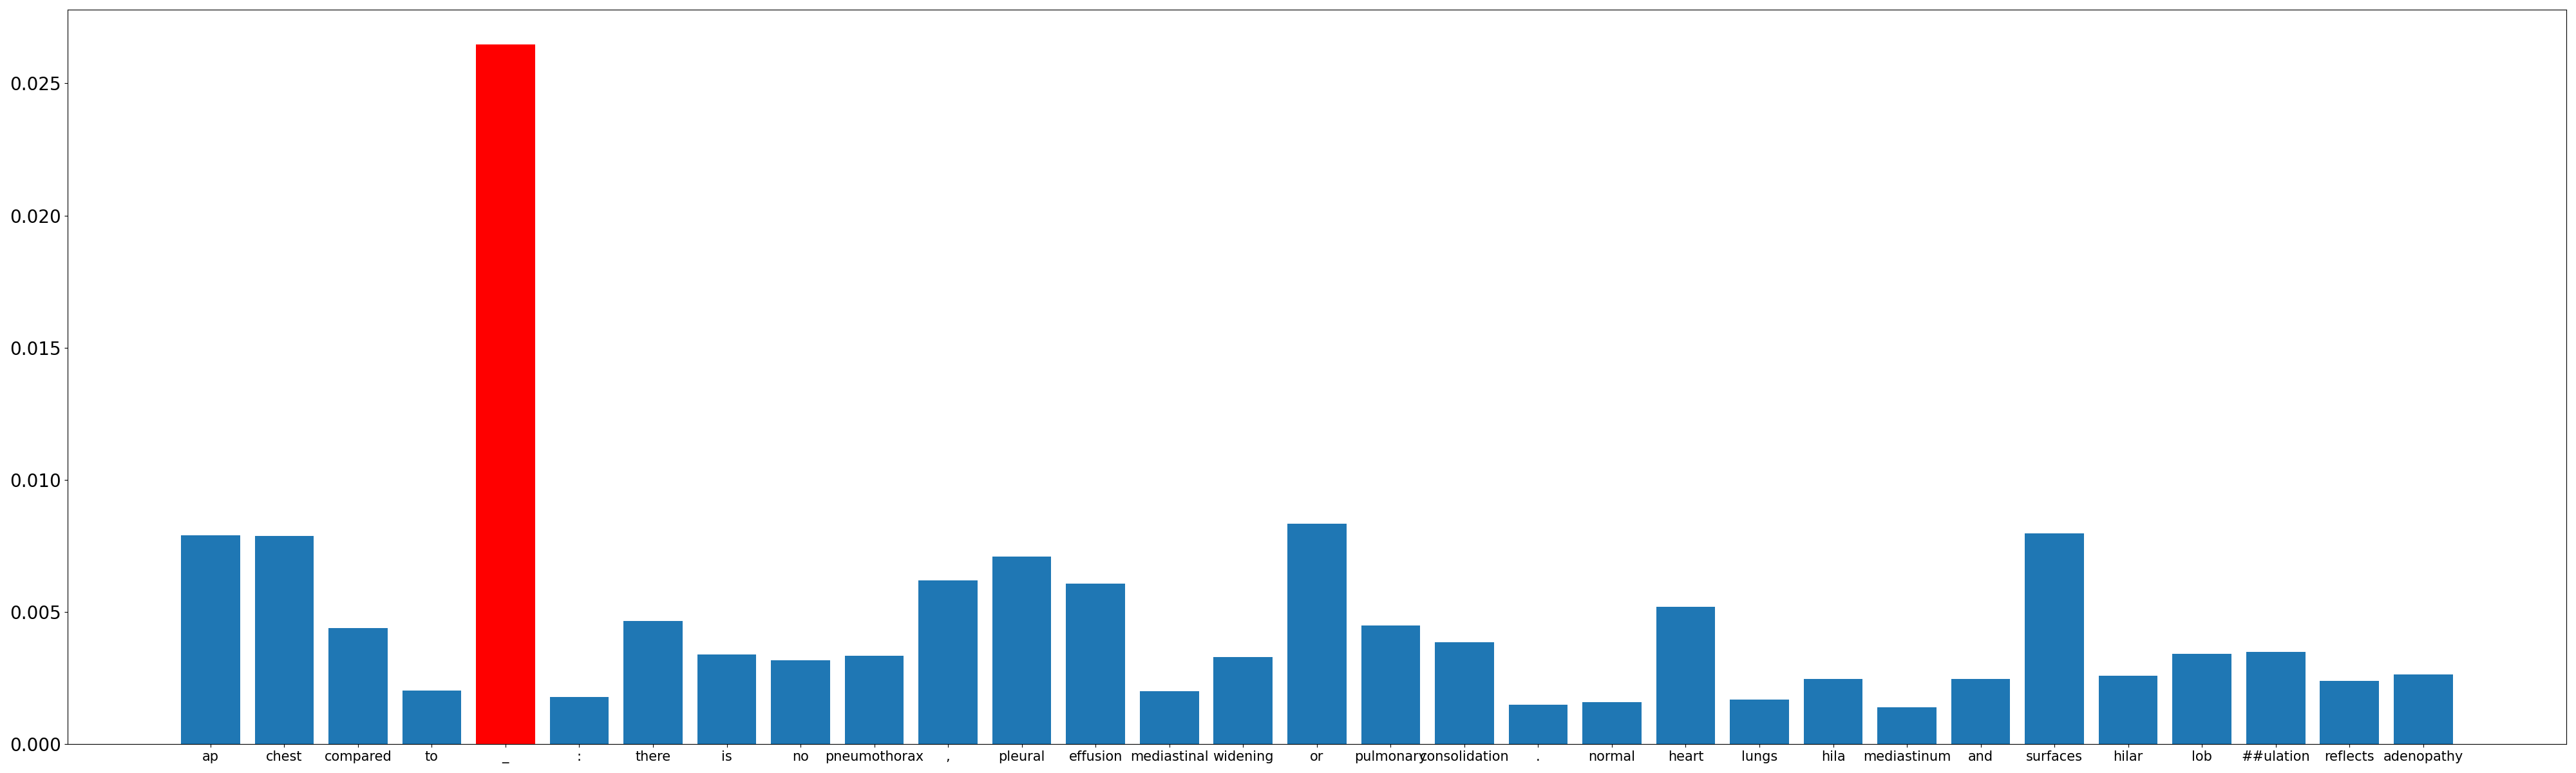}
    }
    
    \caption{Figure illustrating the individual contribution of tokens (text-conditional norm) in memorized prompts. The tokens added for de-identification of PHI (\quotes{\textcolor{red}{\textunderscore\textunderscore\textunderscore}}) hold the most significant contribution towards memorization.}
    \label{fig:three_plots}
\end{figure}

\subsection{Existing Intervention Methods are Ineffective}

Here, we show the ineffectiveness of existing memorization mitigation methods. We plot multiple generations across different seeds for the original \textcolor{red}{memorized} prompt containing the de-identification marker. Next, we modify the prompts by replacing the de-identification token with different mitigation techniques: (1) Random Word Addition, (2) Random Number Addition, and (3) Complete removal. We also plot the average L2 distance between 50 different generations with each prompt. A higher L2 distance indicates more diversity in generations and lesser memorization. \\
\textbf{Qualitatively Analysis:} We observe (Fig. \ref{fig:first}) that replacing or removing the de-identification marker using different strategies remains ineffective in alleviating memorization. \textbf{Quantitatively Analysis: }This is further validated (Fig. \ref{fig:second}) through a minimal change in the mean L2 distance across generations.

\begin{figure}[ht]
    \centering
    % First figure
    \begin{minipage}{\textwidth}
        \centering
        \includegraphics[width=0.8\linewidth]{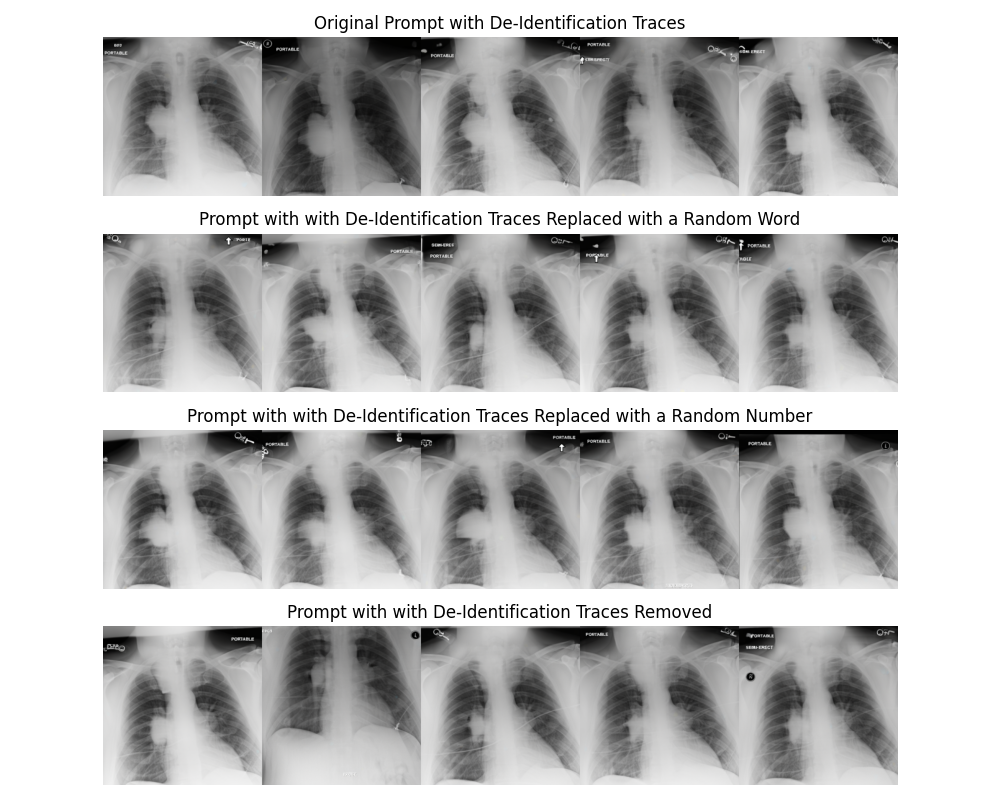}
        \caption{Multiple generations across different seeds with prompt modifications.}
        \label{fig:first}
    \end{minipage}
    \hfill
    % Second figure
    \begin{minipage}{\textwidth}
        \centering
        \includegraphics[width=0.8\linewidth]{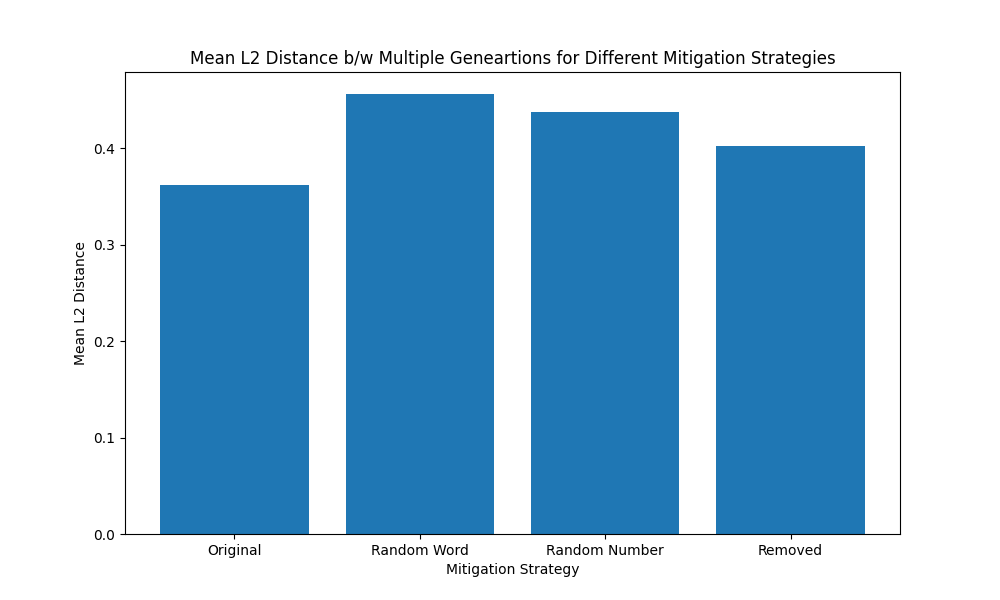}
        \caption{Mean L2 distance across different generations for each prompt.}
        \label{fig:second}
    \end{minipage}
    \caption{Figure illustrating the ineffectiveness of existing (inference-time) memorization mitigation strategies. \\
    \textbf{Figure (a):} Multiple generations across different seeds for the original \textcolor{red}{memorized} prompt (top row) and replacing de-identification marker with a random word (second row), random number (third row), and an empty string (fourth row). In each case, images still show remarkable similarity with one another despite adopting different inference-time memorization mitigation strategies \cite{somepalli2023understanding}. \\
    \textbf{Figure (b):} Comparing the mean L2 distance between different generations using different intervention methods. }
    \label{fig:mitigation_strategies_with_bar_plots}
    
\end{figure}
